# Supplementary material for: 3D Scene Grammar for Parsing RGB-D Pointclouds
Source: arXiv:1211.1752 source file (2012-11-08)
Supplement: Supplementary file 1 [file suplementary.tex]

\documentclass{article} % For LaTeX2e
\usepackage{nips10submit_09,times}
\usepackage{cite}

\usepackage{ upgreek }
\usepackage{verbatim} 

\usepackage{amssymb}
\usepackage{graphicx}
\usepackage{url}
\usepackage{verbatim} 
\usepackage{color}
\usepackage{wrapfig}

\usepackage[numbers]{natbib}
\usepackage{array}
\usepackage{relsize}
\usepackage{multirow}

%%%%%%%%%%%%%%%%%%%%%%%%%%%%%%%%%%%%%%%%%%%%%%%%%%%%%%%%%%%%
% command for hline with varied width
\newlength\savedwidth

%%%%%%%%%%%%%%%%%%%%%%%%%%%%%%%%%%%%%%%%%%%%%%%%%%%%%%%%%%%%

\input{space_saver}

\title{Semantic Labeling of Indoor Environments using RGB-D Images}

\nipsfinalcopy
\begin{document}
\maketitle

\section {Visual Results:}

\subsection{Home Scenes:}

Visual results of our model on a home scene:
  \begin{figure}[h!]
 \centering

\includegraphics[width=\linewidth,height=3.5in]{AAoriginal.eps} 

 \caption{ Pointcloud image of a home (bedroom) scene.}
\label{fig:examplePCD}
 \end{figure}
 
   \begin{figure}[h!]
 \centering

\includegraphics[width=\linewidth,height=3.5in]{AARoomGroundTruth.eps} \\
\includegraphics[width=\linewidth,height=0.2in]{LegendAARoom.eps}\\
 \caption{Ground-truth labels for the above home scene.}
\label{fig:examplePCD}
 \end{figure}
 
   \begin{figure}[h!]
 \centering

\includegraphics[width=\linewidth,height=3.5in]{AARoomPredicted.eps} \\
\includegraphics[width=\linewidth,height=0.2in]{LegendAARoom.eps}
 \caption{Predicted labels for the above home scene.}
\label{fig:examplePCD}
 \end{figure}
 
 \clearpage
\pagebreak
\subsection{Office Scenes:}
Visual results of our model on an office scene:
 \begin{figure}[h!]
 \centering
\includegraphics[width=\linewidth,height=3in]{5150Original.eps} 
 \caption{Pointcloud image of an office scene}
\label{fig:examplePCD}
 \end{figure}
 
   \begin{figure}[h!]
 \centering
\includegraphics[width=\linewidth,height=3in]{5150GroundTruth.eps} \\
 \includegraphics[width=\linewidth,height=0.2in]{LegendMengLab.eps}
 \caption{Ground-truth labels for the above office scene}
\label{fig:examplePCD}
 \end{figure}
 
   \begin{figure}[h!]
 \centering
\includegraphics[width=\linewidth,height=3in]{5150labeled.eps} \\
 \includegraphics[width=\linewidth,height=0.2in]{LegendMengLab.eps}
 \caption{Predicted labels for the above office scene.}
\label{fig:examplePCD}
 \end{figure}

\clearpage
  \newpage
\section {Confusion Matrices:}
 \subsection{Home Scenes:}
 
   \begin{figure}[h!] 
 \centering
 \includegraphics[scale=0.25]{ConfusionFinal/home/nodeonly_imagefeats.csv.eps} 
 \caption{Confusion Matrix on home dataset with svm\_nodeonly trained on Image features }
\label{fig:confusionMatrix}
 \end{figure}

 \begin{figure}[h!]   
 \centering
 \includegraphics[scale=0.25]{ConfusionFinal/home/nodeonly_pcfeats.csv.eps} 
 \caption{Confusion Matrix on home dataset with svm\_nodeonly trained on Shape features }
\label{fig:confusionMatrix}
 \end{figure}

  \begin{figure}[h!]   
 \centering
 \includegraphics[scale=0.25]{ConfusionFinal/home/nodeonly_allfeats.csv.eps} 
 \caption{Confusion Matrix on home dataset with svm\_nodeonly trained on Shape and Image features }
\label{fig:confusionMatrix}
 \end{figure}
 
   \begin{figure}[h!]   
 \centering
 \includegraphics[scale=0.25]{ConfusionFinal/home/assoc_radius0.6.csv.eps} 
 \caption{Confusion Matrix on home dataset with svm\_mrf\_assoc trained on Shape and Image features }
\label{fig:confusionMatrix}
 \end{figure}
 
  \begin{figure}[h!]   
 \centering
 \includegraphics[scale=0.25]{ConfusionFinal/home/nonassoc_radiu0.6.csv.eps} 
 \caption{Confusion Matrix on home dataset with svm\_mrf\_nonassoc trained on Shape and Image features }
\label{fig:confusionMatrix}
 \end{figure}
 
  \begin{figure}[h!]   
 \centering
 \includegraphics[scale=0.25]{ConfusionFinal/home/objassoc_radiu0.6.csv.eps} 
 \caption{Confusion Matrix on home dataset with svm\_mrf\_parsimon trained on Shape and Image features }
\label{fig:confusionMatrix}
 \end{figure}
 
 \clearpage
  \newpage
\subsection{Office Scenes:}
  \begin{figure}[h!] 
 \centering
 \includegraphics[scale=0.25]{ConfusionFinal/office/nodeonly_imagefeats.csv.eps} 
 \caption{Confusion Matrix on office dataset with svm\_nodeonly trained on Image features }
 \label{fig:confusionMatrix}
 \end{figure}

   \begin{figure}[h!] 
\centering
 \includegraphics[scale=0.25]{ConfusionFinal/office/nodeonly_pcfeats.csv.eps} 
 \caption{Confusion Matrix on office dataset with svm\_nodeonly trained on Shape features }
 \label{fig:confusionMatrix}
 \end{figure}
 
   \begin{figure}[h!] 
  
   \begin{minipage}[b]{\linewidth}
 \centering
 \includegraphics[scale=0.25]{ConfusionFinal/office/nodeonly_allfeats.csv.eps} 
 \caption{Confusion Matrix on office dataset with svm\_nodeonly trained on Shape and Image features }
  \end{minipage}
\label{fig:confusionMatrix}
 \end{figure}
 
   \begin{figure}[h!]   
 \centering
 \includegraphics[scale=0.25]{ConfusionFinal/office/assoc_radius0.6.csv.eps} 
 \caption{Confusion Matrix on office dataset with svm\_mrf\_assoc trained on Shape and Image features }
\label{fig:confusionMatrix}
 \end{figure}
 
  \begin{figure}[h!]   
 \centering
 \includegraphics[scale=0.25]{ConfusionFinal/office/nonassoc_radius0.6.csv.eps} 
 \caption{Confusion Matrix on office dataset with svm\_mrf\_nonassoc trained on Shape and Image features }
\label{fig:confusionMatrix}
 \end{figure}
 
  \begin{figure}[h!]   
 \centering
 \includegraphics[scale=0.25]{ConfusionFinal/office/objassoc_radius0.6.csv.eps} 
 \caption{Confusion Matrix on office dataset with svm\_mrf\_parsimon trained on Shape and Image features }
\label{fig:confusionMatrix}
 \end{figure}
 \clearpage
  \newpage

\end{document}
